# Supplementary material for: Learning and Retrieval from Prior Data for Skill-based Imitation Learning
Source: arXiv:2210.11435 source file (2022-11-15)
Supplement: Supplementary file 1 [file qual-analysis.tex]

\section{Supplementary Video}
\label{app:qual-analysis}

\textbf{Please refer to the supplementary videos} for visualizations of our datasets, comparisons of our method and baselines, and visualizations of sub-trajectories retrieved by our method.
